# Supplementary material for: Asymmetric Berry-Phase Interference Patterns in a Single-Molecule Magnet
Source: arXiv:1106.0258 source file (2011-06-01)
Supplement: Supplementary file 1 [file Qudussi_supplementary_information.pdf]

# Supplementary information

## Asymmetric Berry-Phase Interference Patterns in a Single-Molecule Magnet

H. M. Quddusi[1], J. Liu[2], S. Singh[1], K. J. Heroux[4], E. del Barco[1], S. Hill[3], and D. N. Hendrickson[4]

[1]*Department of Physics, University of Central Florida, Orlando, FL 32816, USA*

[2]*Department of Physics, University of Florida, Gainesville, FL 32611, USA*

[3]*National High Magnetic Field Laboratory and Department of Physics, Florida State University, Tallahassee, FL 32310, USA and*

[4]*Department of Chemistry and Biochemistry, University of California at San Diego, La Jolla, CA 92093, USA*

Figure S1 shows the temperature dependence of EPR spectra obtained at 139.5GHz with the applied field close to the molecular easy axis. Peak assignments can be made on the basis of the temperature dependence of the resonances and their relative spacings (for further details, see Ref. [1]). Those resonances belonging to the $S = 9$ ground state have been labeled in the figure (A resonances, with the subscript denoting the absolute value of the spin projection associated with the level from which the transition was excited). Careful examination of the 20 K spectrum reveals nine successive peaks belonging to the A series, distributed from 1.15 T to ~4.75 T, which is just below the $g = 2.00$ position for 139.5 GHz. This confirms that the molecule processes an $S = 9$ spin ground state. The intensity of the $A_9$ transition increases as the temperature decreases, indicating that it is the ground state transition, i.e., $m_S = -9$ to $-8$. Additional resonances are observed at elevated temperatures, confirming the existence of many low-lying excited spin ($S < 9$) multiplets. Simulations (see below) reveal the presence of many overlapping excited spin states not far above the lowest lying levels associated with the $S = 9$ ground state ($m_S = -9$ and $-8$), making assignment of the excited state resonances essentially impossible. The existence of the low-lying excited states is consistent with the relatively weak exchange coupling within the magnetic core of the molecule. We note that almost identical spectra have been obtained for a related $Mn_4$ complex, albeit with slightly enhanced coupling, resulting in a reduced density of low-lying excited spin states [1]. Thus, comparison between the spectra obtained for the two complexes provides added support to the assignments made in Fig. S1.

Figure S2 shows the frequency dependence of the A resonance peak positions obtained with the field approximately parallel (within a few degrees) to the molecular easy axis. The solid lines in the figure represent simulations of the EPR transitions within the $S = 9$ ground state; they have been color coded to denote the associated transitions. For some frequencies, many resonances are observed, because the measurements were performed at an elevated temperature (20 K); meanwhile, measurements were performed at a low temperature of 3 K for those frequencies where only one or two resonances are plotted. The simulations were performed employing the Hamiltonian and parameters given in the main text. Simultaneous constraints were provided by the A series of EPR peaks (Fig. S2), as well as the main features

of the hysteresis measurements presented in the main text. As shown in Fig. S2, the simulations are in excellent agreement with all of the ground state EPR transitions.

[1] J. Liu et al., Polyhedron, in press.

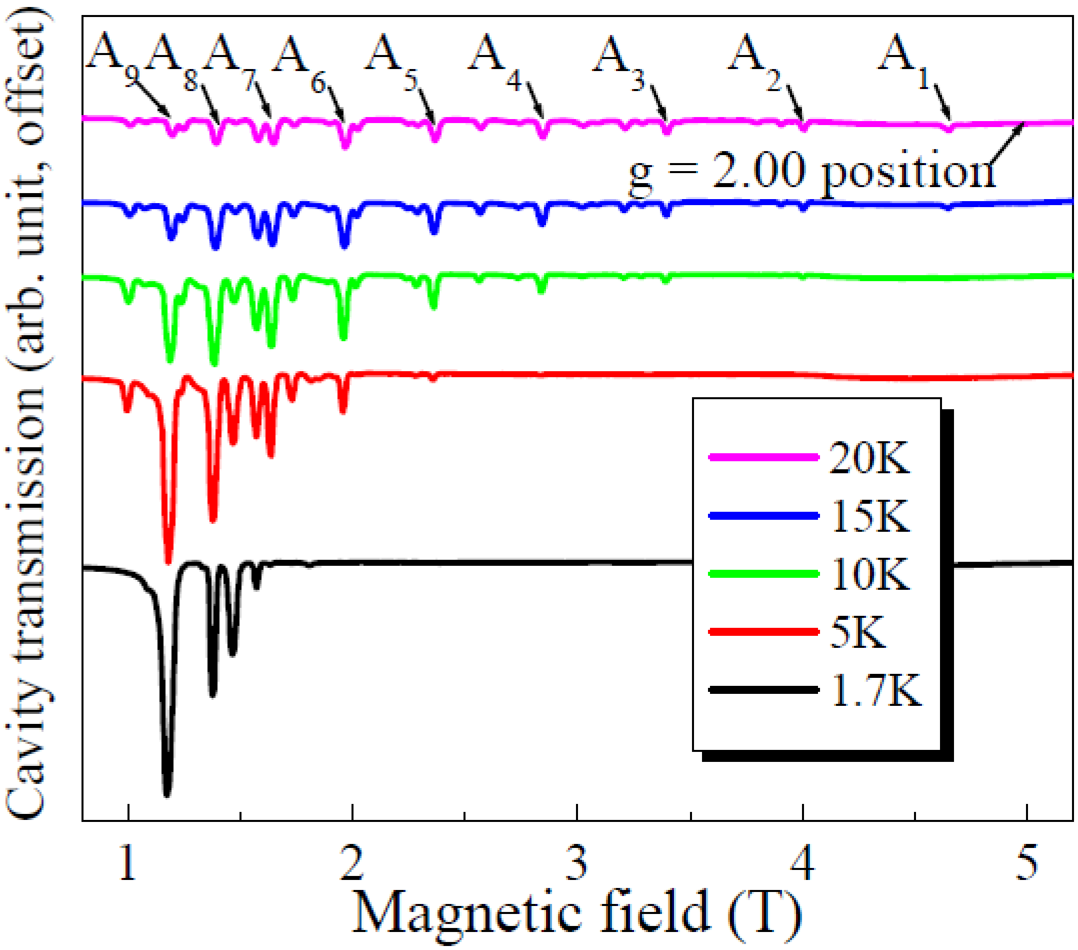


Fig. S1. Temperature dependent EPR spectra obtained at 139.5 GHz with the applied field close to the molecular easy-axis. The transition peaks $A_1$, $A_2$…$A_9$ represent transitions within the *S* = 9 ground state multiplet.

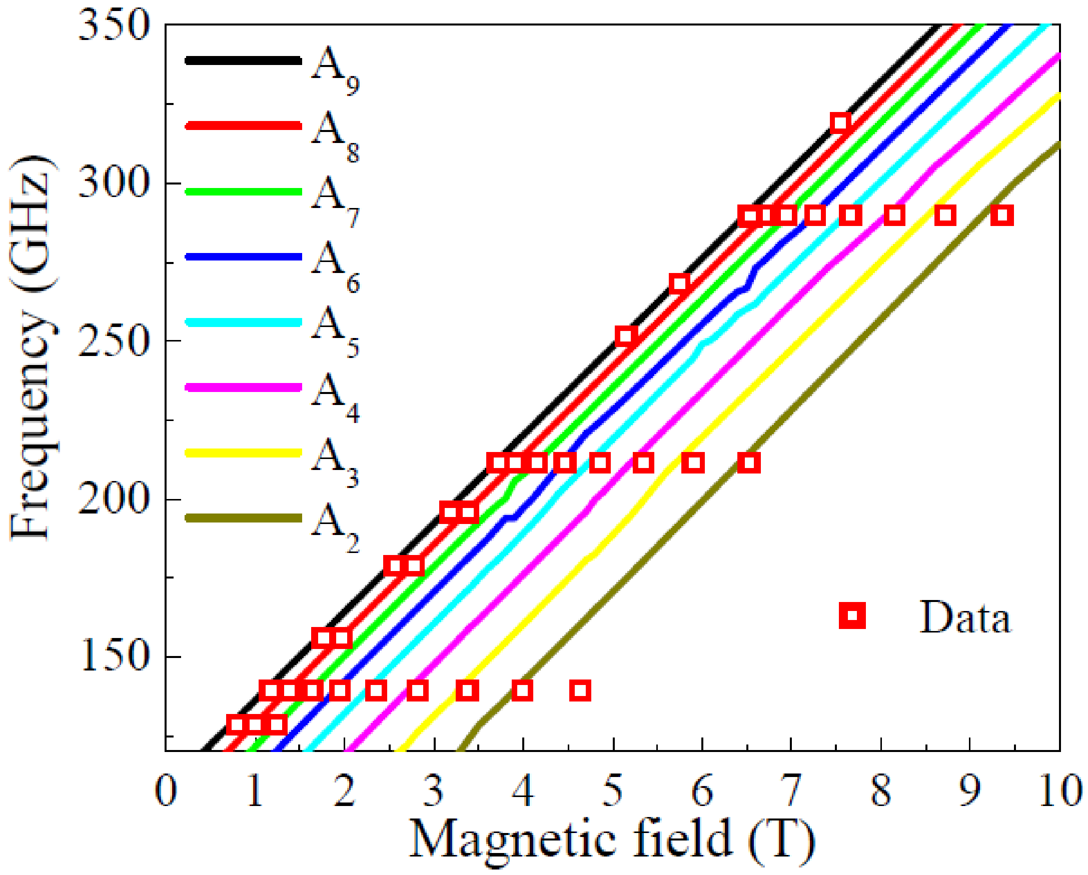


Fig. S2. Plot of frequency versus field showing the observed ground state EPR peak positions, with the applied field close to the molecular easy-axis. Low-temperature data were collected at 3 K, while additional temperature dependence studies were performed at 139.5 GHz, 211.4 GHz and 289.6 GHz. The solid lines are the simulations of A series peak positions (red squares) using the Hamiltonian and parameters provided in the main text.
